# Supplementary material for: Verifiable Differential Privacy
Source: arXiv:2208.09011 source file (2023-01-20)
Supplement: Supplementary file 1 [file d_misc.tex]

\section{Discrete Log Assumption}
\label{sec: DLG}
The discrete log game consists of interactions between a challenger and an adversary PPT $\mathcal{A}$. The game proceeds as follows:

\begin{enumerate}
    \item{The challenger samples $x \xleftarrow[]{R} \Z_q$ and computes $h= g^x$}
    
    \item{The challenger sends $h, g$ to $\mathcal{A}$ over a secure authenticated channel}
    
    \item{The adversary tries to guess $x$ by outputting $\hat{x}$}
\end{enumerate}

We define the advantage of the adversary as the probability of guessing $x$ correctly i.e. 
$$\adv(\mathcal{A}, \G) := \prob{\hat{x}=x}$$

The discrete log assumption states that for all probabilistic polynomial time adversaries $\mathcal{A}$, $\adv(\mathcal{A}, \G) = \mu(q)$ where $\mu$ is negligble in $q$.
